# Supplementary material for: Hidden symmetries, instabilities, and current suppression in Brownian ratchets
Source: arXiv:1512.07802 source file (2015-12-24)
Supplement: Supplementary file 1 [file SI.pdf]

# Supplementary Information
# Hidden symmetries, instabilities, and current suppression in Brownian ratchets

David Cubero[1] and Ferruccio Renzoni[2]
[1] *Departamento de Física Aplicada I, EPS, Universidad de Sevilla, Calle Virgen de África 7, 41011 Sevilla, Spain and*
[2] *Department of Physics & Astronomy, University College London, Gower Street, London WC1E 6BT, UK*
(Dated: November 13, 2015)

## I. Hidden symmetries in a 1D overdamped system

An overdamped Brownian particle subject to a periodic potential of spatial period $L$, $U(x+L)=U(x)$ for all $x$, and a periodic driving force of temporal period $\tau$, $F(t+\tau)=F(t)$ for all $t$, has a probability density $P(x,t)$ determined by the Smoluchowski equation, [1],

$$\frac{\partial P}{\partial t}=D\frac{\partial^2 P}{\partial x^2}-\frac{1}{\gamma}\frac{\partial}{\partial x}\left(-\frac{\partial V}{\partial x}P+F(t)P\right), \qquad \text{(S.1)}$$

where $D=\Gamma/\gamma^2$ is the diffusion constant, $\Gamma$ is the noise strength, and $\gamma$ the friction coefficient. We show here that the average velocity $\langle v\rangle=\lim_{t\to\infty}\langle x(t)\rangle/t$ is invariant under the following transformations:

$$\hat{S}_1: F(t)\to F(-t), \qquad \text{(S.2)}$$

$$\hat{S}_2: f(x)\to f(-x), \qquad \text{(S.3)}$$

where $f(x)=-\partial U/\partial x$ is the conservative, static force. In addition, at the end of the section we prove that the average velocity of an overdamped particle in a one-dimensional system under the more general time-dependent force $\mathcal{F}(x,t)=-\partial U(x,t)/\partial x$—a setup that includes flashing ratchets—is invariant under the following symmetry transformation

$$\hat{S}_3: \mathcal{F}(x,t)\to\mathcal{F}(-x,-t). \qquad \text{(S.4)}$$

In systems driven by time-dependent forces, i.e. $\mathcal{F}(x,t)=f(x)+F(t)$, invariance under both transformations $\hat{S}_1$ and $\hat{S}_2$ implies invariance under $\hat{S}_3$, but the reverse in general does not hold.

To prove the invariance under the abovelisted transformations, it is convenient to introduce the reduced probability density $\hat{P}(x,t)$, defined by

$$\hat{P}(x,t)=\sum_{n=-\infty}^{\infty}P(x+nL,t)\ . \qquad \text{(S.5)}$$

$\hat{P}(x,t)$ obeys the same equation (S.1) but it is also space periodic. Assuming that the driving force is unbiased

$$\int_0^\tau dt\, F(t)=0, \qquad \text{(S.6)}$$

the current can be expressed in terms of the reduced probability density as [2]

$$\langle v\rangle=\lim_{t\to\infty}\frac{1}{t}\int_0^t dt'\int_0^L dx\hat{P}(x,t')\frac{f(x)}{\gamma}. \qquad \text{(S.7)}$$

In order to compute the current we are interested in the asymptotic attractor solution to which all solutions converge in the long time limit. This asymptotic solution is periodic in time. Hence we can Fourier expand in time and space the probability density as

$$\hat{P}(x,t)=\sum_{n=-\infty}^{\infty}\sum_{m=-\infty}^{\infty}P_n^{(m)}e^{in\omega t}e^{imkx}, \qquad \text{(S.8)}$$

where $P_n^{(m)}$ are the Fourier coefficients and $\omega=2\pi/\tau$, $k=2\pi/L$. The normalization of the reduced probability density implies

$$P_n^{(0)}=\frac{\delta_{n,0}}{L}. \qquad \text{(S.9)}$$

From Eq. (S.7), the current is written as

$$\langle v\rangle=\frac{1}{\tau}\int_0^\tau dt'\int_0^L dx\hat{P}(x,t')\frac{f(x)}{\gamma}=\frac{L}{\gamma}\sum_m P_0^{(m)}f^{(-m)}, \qquad \text{(S.10)}$$

where $f^{(m)}$ are the Fourier coefficients of the static conservative force

$$f^{(m)}=\frac{1}{L}\int_0^L dx\, e^{-imkx}f(x). \qquad \text{(S.11)}$$

Introducing the expansion (S.8) into (S.1) yields the following linear system for the Fourier coefficients $P_n^{(m)}$,

$$\sum_{n'=-\infty}^{\infty}\sum_{m'=-\infty}^{\infty}\mathcal{S}_{n,n'}^{m,m'}P_{n'}^{(m')}=0, \qquad \text{(S.12)}$$

where

$$\mathcal{S}_{n,n'}^{m,m'}=\left(in\omega+Dm^2k^2\right)\delta_{n,n'}\delta_{m,m'}+\frac{ikm}{\gamma}\left[F_{n-n'}\delta_{m,m'}+f^{(m-m')}\delta_{n,n'}\right], \qquad \text{(S.13)}$$

and $F_n$ are the Fourier coefficients of the driving force $F(t)$,

$$F_n=\frac{1}{\tau}\int_0^\tau dt\, e^{-in\omega t}F(t). \qquad \text{(S.14)}$$

A pair of indices formed by one spatial index $m$ and one temporal index $n$ can always be mapped into a single index $j$. Thus, the linear problem (S.12) can be seen as an

ordinary linear system for the set of variables $P_j = P_n^{(m)}$. However, since (S.12) is an homogeneous system of linear equations and there must exist a non-trivial solution, we conclude the matrix $S$ is not invertible. The problem can be recast as an inhomogeneous linear problem, with the inhomogeneous part determined by the normalization condition (S.9). By excluding all points with $m = 0$ the problem can be recast as

$$\sum_{n'} \sum_{m' \neq 0} \mathcal{M}_{n,n'}^{m,m'} P_{n'}^{(m')} = \mathcal{D}_n^{(m)}, \tag{S.15}$$

where the indexes run over the values $m = \pm 1, \pm 2, \ldots$, $n = 0, \pm 1, \ldots$. The invertible matrix $\mathcal{M}$ is given by

$$\mathcal{M}_{n,n'}^{m,m'} = \left( \frac{in\omega}{m} + Dmk^2 \right) \delta_{n,n'} \delta_{m,m'} + \frac{ik}{\gamma} \left[ F_{n-n'} \delta_{m,m'} + f^{(m-m')} \delta_{n,n'} \right]. \tag{S.16}$$

and the inhomogeneous term is

$$\mathcal{D}_n^{(m)} = -\frac{1}{L} \mathcal{S}_{n,0}^{(m,0)} = -\frac{ik}{L\gamma} f^{(m)} \delta_{n,0}. \tag{S.17}$$

This problem can be numerically solved by using standard numerical algorithms for sparse linear systems if we truncate the Fourier expansions to sufficiently large numbers $M$ and $N$, i.e. $m = \pm 1, \pm 2, \ldots, \pm M$ and $n = 0, \pm 1, \ldots \pm N$. Thus, in this truncated problem the single index runs over the values $j = 1, 2, \ldots, 2M(2N+1)$.

Solving the linear system is equivalent to finding the inverse matrix of $\mathcal{M}$. Denoting by $\mathcal{N}$ such an inverse matrix

$$\sum_{l \neq 0} \sum_s \mathcal{N}_{n,s}^{m,l} \mathcal{M}_{s,n'}^{l,m'} = \sum_{l \neq 0} \sum_s \mathcal{M}_{n,s}^{m,l} \mathcal{N}_{s,n'}^{l,m'} = \delta_{m,m'} \delta_{n,n'}, \tag{S.18}$$

then the solution $P_n^{(m)}$ is

$$P_n^{(m)} = \sum_{m' \neq 0} \sum_{n'} \mathcal{N}_{n,n'}^{m,m'} D_{n'}^{(m')} = -\frac{ik}{\gamma L} \sum_{m' \neq 0} \mathcal{N}_{n,0}^{m,m'} f^{(m')}. \tag{S.19}$$

We are now in a position to discuss the invariance under the transformations (S.2) and (S.3). The transformation

$$\hat{S}_1 : \quad F(t) \to \widetilde{F}(t) = F(-t) \tag{S.20}$$

is equivalent to replace $F_n \to \widetilde{F}_n = F_{-n}$. Thus, the transformed probability density $\widetilde{P}$ is determined by the transformed matrix $\widetilde{\mathcal{M}}$

$$\hat{S}_1 : \quad \mathcal{M}_{n,n'}^{m,m'} \to \widetilde{\mathcal{M}}_{n,n'}^{m,m'} = \mathcal{M}_{n',n}^{m,m'}. \tag{S.21}$$

This last equation express the transformation $\hat{S}_1$ as a transposition of the time indexes $n$ and $n'$ in the matrix $\mathcal{M}$. In order to compute the inverse, it is convenient to express (S.18) with the following matrix notation

$$\sum_{l \neq 0} \mathcal{N}^{m,l} \mathcal{M}^{l,m'} = \sum_{l \neq 0} \mathcal{M}^{m,l} \mathcal{N}^{l,m'} = \delta_{m,m'} I_N, \tag{S.22}$$

where $\mathcal{N}^{m,m'}$, $\mathcal{M}^{m,m'}$ and $I_N$ are matrices of order $(2N+1) \times (2N+1)$, and the latter is the identity matrix $(I_N)_{n,n'} = \delta_{n,n'}$. By applying the transpose operation to (S.22)

$$\sum_{l \neq 0} (\mathcal{M}^{m,l})^t (\mathcal{N}^{l,m'})^t = \sum_{l \neq 0} (\mathcal{N}^{m,l})^t (\mathcal{N}^{l,m'})^t = \delta_{m,m'} I_N. \tag{S.23}$$

The matrix $M^{m,l}$ with $l \neq m$ is proportional to the indentity matrix $I_N$, $M_{n,n'}^{m,l} = (ik/\gamma) f^{m-l} \delta_{n,n'}$, thus, $M^{m,l}$ commutes with all $N^{l,m'}$. Assuming that also $M^{m,m}$ commutes with $N^{m,m'}$, as it will be shown in the following, we arrive to

$$\hat{S}_1 : \quad \mathcal{N}_{n,n'}^{m,m'} \to \widetilde{\mathcal{N}}_{n,n'}^{m,m'} = \mathcal{N}_{n',n}^{m,m'}, \tag{S.24}$$

which, using (S.19) yields

$$\hat{S}_1 : \quad P_0^{(m)} \to \widetilde{P}_0^{(m)} = -\frac{ik}{\gamma L} \sum_{m' \neq 0} \mathcal{N}_{0,0}^{m,m'} f^{(m')} = P_0^{(m)}. \tag{S.25}$$

Using this result in (S.10), we prove the invariance of the average velocity under the transformation $F(t) \to F(-t)$.

The proof of the current's invariance under the transformation

$$\hat{S}_2 : \quad f(x) \to \widetilde{f}(x) = f(-x) \tag{S.26}$$

proceeds in a similar fashion. First we notice that this transformation is equivalent to the transformation $f^{(m)} \to f^{(-m)}$ for the Fourier coefficients of the static force, and thus to a transposition of the space indexes of the matrix $\mathcal{M}_{n,n'}^{m,m'} \to \mathcal{M}_{n,n'}^{m',m}$. By operating as before, we find

$$\hat{S}_2 : \mathcal{N}_{n,n'}^{m,m'} \to \mathcal{N}_{n,n'}^{m',m}, \tag{S.27}$$

after the assumption that the matrixes $\mathcal{M}_{n,n}$—of order $2M \times 2M$—commute with $\mathcal{N}_{n',n}$ for all $n$ and $n'$, and thus

$$\hat{S}_2 : \quad P_0^{(m)} \to -\frac{ik}{\gamma L} \sum_{m' \neq 0} \mathcal{N}_{0,0}^{m',m} f^{(-m')}, \tag{S.28}$$

which in general is different from the original coefficient $P_0^{(m)}$, but yields the same average velocity

$$\langle \widetilde{v} \rangle = -\frac{ik}{\gamma^2} \sum_{m \neq 0} \sum_{m' \neq 0} \mathcal{N}_{0,0}^{m',m} f^{(-m')} f^{(m)} = -\frac{ik}{\gamma^2} \sum_{m \neq 0} \sum_{m' \neq 0} \mathcal{N}_{0,0}^{m,m'} f^{(m')} f^{(-m)} = \langle v \rangle. \tag{S.29}$$

The symmetries $\hat{S}_1$ and $\hat{S}_2$ imply each other, as we show in the following. By taking into account the definition of $\mathcal{N}$, i.e. by substracting the middle side to the lefthand side of (S.18), we obtain,

$$\left( \mathcal{M}^{m,m} \mathcal{N}^{m,m'} - \mathcal{N}^{m,m'} \mathcal{M}^{m,m} \right)_{n,n'} = - \left( \mathcal{M}_{n',n'} \mathcal{N}_{n,n'} - \mathcal{N}_{n,n'} \mathcal{M}_{n',n'} \right)^{m,m'}. \tag{S.30}$$

Therefore, $\mathcal{M}^{m,m}$ only commutes with $\mathcal{N}^{m,m'}$, and thus symmetry $\hat{S}_1$ is satisfied, if and only if $\mathcal{M}_{n,n}$ commutes with $\mathcal{N}_{n',n}$—i.e. the symmetry $\hat{S}_2$ holds.

We conclude by showing that the matrixes $\mathcal{M}^{m,m}$ commute with $\mathcal{N}^{m',m}$. A matrix formed by repeated matrix multiplication of $\mathcal{M}^{m,m}$, i.e. $(\mathcal{M}^{m,m})^k$ with $k$ integer, does commute with $\mathcal{M}^{m,m}$, regardless of the specific value of $k$. It is easy to show that for the specific form (S.16) of the infinite-dimensional matrix $\mathcal{M}$, the $k$th-power $(\mathcal{M}^{m,m})^k$ is linearly independent of all other powers, thus we can expand an arbitrary matrix of order $(2N+1)\times(2N+1)$ as a linear combination of these power matrixes. In particular, we are interested in the solution of our linear problem $\mathcal{N}^{m',m}$, which is expanded as

$$\mathcal{N}^{m',m} = \sum_{k=0}^{N_k} \lambda_k^{m',m} (\mathcal{M}^{m,m})^k, \tag{S.31}$$

where $\lambda_k^{m',m}$ are complex coefficients and $N_k = (2N+1)^2 - 1$. Notice that by $(\mathcal{M}^{m,m})^k$ we do not refer to the power matrixes obtained by matrix multiplication of a truncated matrix $\mathcal{M}^{m,m}$ of order $(2N+1)\times(2N+1)$, but to the (truncated) power matrixes that result from multiplying the (untruncated) matrixes $\mathcal{M}^{m,m}$ as given by (S.16). These latter power matrixes, despite being defined in a space of infinite dimension, are straightforward to compute, and, being the multiplication not affected by the truncation of the matrix, different from the former. We are thus not limited by the Cayley-Hamilton theorem, which states that an arbitrary square matrix $\mathcal{A}$ of order $(2N+1)\times(2N+1)$ satisfies its own characteristic equation—and therefore the power matrix $\mathcal{A}^{2N+1}$ is a linear combination of the lower matrix powers of $\mathcal{A}$. In the infinite space, all powers of $(\mathcal{M}^{m,m})^k$ are linearly independent of each other.

Inserting Eq. (S.31) into Eq. (S.22) yields the linear system

$$\sum_{k=0}^{N_k} \sum_{l=-M, l\neq 0}^{M} \lambda_k^{m',l} \mathcal{M}^{m,l} (\mathcal{M}^{l,l})^k = \delta_{m,m'} I_N. \tag{S.32}$$

Since the power matrixes are independent, the linear problem (S.32) has a unique solution for the coefficients $\lambda_k^{m',l}$, and the inverse matrix $\mathcal{N}^{m',m}$ can indeed be written in the form (S.31), which obviously commutes with $\mathcal{M}^{m,m}$. This holds for any $N$ and $M$, and thus also in the limit $N, M \to \infty$.

In a two-dimensional system the corresponding matrixes $\mathcal{M}^{mq,mq}$, with $m$ and $q$ the Fourier indices in orthogonal directions, can be written as a linear combination of matrices of the same kind,

$$\mathcal{M}^{mq,mq} = \mathcal{M}^{m0,m0} + \mathcal{M}^{0q,0q} - \mathcal{M}^{10,10} - \mathcal{M}^{01,01} + \mathcal{M}^{11,11}. \tag{S.33}$$

Therefore, they are not linearly independent, and in general the solution matrix $\mathcal{N}$ cannot be expanded as a linear combination of these matrixes. This prevents the generalisation of the above proof to higher dimensions, hence the hidden symmetries (S.2)–(S.3) do not in general hold in higher dimensions.

### A. A more general time-dependent potential

We now consider an overdamped particle in a one-dimensional system subject to a more general time-dependent force $\mathcal{F}(x,t) = -\partial U(x,t)/\partial x$. The current is generalized from (S.10) to

$$\langle v \rangle = \frac{L}{\gamma} \sum_m \sum_n P_n^{(m)} F_{-n}^{(-m)}, \tag{S.34}$$

where $F_n^{(m)}$ are the Fourier coefficients of the total force

$$F_n^m = \frac{1}{L\tau} \int_0^L dx \int_0^\tau dt\, e^{-i(n\omega t + mkx)} \mathcal{F}(x,t). \tag{S.35}$$

The matrix $\mathcal{M}$ is given by

$$\mathcal{M}_{n,n'}^{m,m'} = \left( \frac{in\omega}{m} + Dmk^2 \right) \delta_{n,n'} \delta_{m,m'} + \frac{ik}{\gamma} F_{n-n'}^{(m-m')}, \tag{S.36}$$

with $m, m' \neq 0$, and the following inhomogeneous term

$$\mathcal{D}_n^{(m)} = -\frac{ik}{L\gamma} F_n^{(m)}, \tag{S.37}$$

which yields the following average velocity

$$\langle v \rangle = \frac{1}{\gamma} F_0^{(0)} - \frac{ik}{L\gamma} \sum_{m,m'\neq 0} \sum_{n,n'} \mathcal{N}_{n,n'}^{(m,m')} F_{-n}^{(-m)} F_{n'}^{(m')}. \tag{S.38}$$

The transformation

$$\hat{S}_3 : \mathcal{F}(x,t) \to \widetilde{\mathcal{F}}(x,t) = \mathcal{F}(-x,-t), \tag{S.39}$$

leads to the transformed matrix $\widetilde{\mathcal{M}}$,

$$\hat{S}_3 : \quad \mathcal{M}_{n,n'}^{m,m'} \to \widetilde{\mathcal{M}}_{n,n'}^{m,m'} = \mathcal{M}_{n',n}^{m',m}. \tag{S.40}$$

The inverse matrix $\widetilde{\mathcal{N}}$ is given by the transposed of the original matrix $\mathcal{N}$,

$$\hat{S}_3 : \quad \mathcal{N}_{n,n'}^{m,m'} \to \widetilde{\mathcal{N}}_{n,n'}^{m,m'} = \mathcal{N}_{n',n}^{m',m}. \tag{S.41}$$

By simple inspection of Eq. (S.38), the invariance of the current under this transformation is proved.

## II. Instability of the time-reversed solution

Given a solution $x(t)$ of the Langevin equation in the overdamped regime,

$$\gamma \dot{x} = f(x) + F(t) + \xi(t), \tag{S.42}$$

if the potential is shift-symmetric, $f(x+L/2) = -f(x)$, and the driving anti-symmetric, $F(-t+t') = -F(t)$, with $t'$ a constant, then the time-reversed trajectory $\widetilde{x}(t) = x(-t+t') + L/2$ is also a solution of the same equation, corresponding to the transformed random force $\widetilde{\xi}(t) = -\xi(-t+t')$, and carrying current in the opposite direction than $x(t)$.

However, this solution is unstable and cannot thus be taken to contribute to the average velocity with the same weigth as the direct trajectory $x(t)$, as assumed in the standard symmetry analysis [3]. A simple confirmation of the instability of this solution is obtained by inspecting the Smoluchowski equation (S.1). For a finite amount of noise $D$, given a solution $P(x,t)$ of the Smoluchowski equation (S.1), the transformed probability density $P(x+L/2, -t+t')$ is not a solution of (S.1) unless $D = 0$, i.e. in a noiseless system.

Even in a noiseless system, the transformed trajectories $\widetilde{x}(t)$ are difficult to observe numerically or in a experiment, since they are unstable and any small perturbation—however weak—makes the system deviate from them. This is illustrated in Figs. S1 and S2.

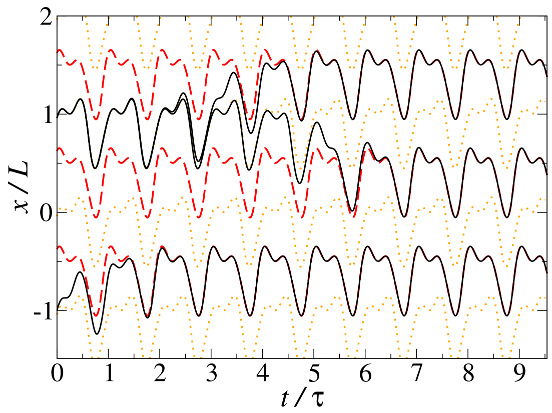


FIG. S1. Instability of the time-reversed solution in a deterministic 1D overdamped system. The potential and drive are $U(x) = U_0 \cos(kx)$ and $F(t) = A[\cos(\omega t) + \cos(2\omega t + \pi/2)]$, which are shift-symmetric and anti-symmetric, respectively. Reduced units are defined such that $m = k = \omega = 1$. Other parameters are $U_0 = \gamma = 50$, $A = 2\gamma$, $\Gamma = 0$. The red dashed lines depict the periodic, attractor solutions $x_0(t)$—which are oscillations about the potential minima. The orange dashed lines correspond to the time-reversed solutions $\widetilde{x}(t) = x_0(-t+\pi) + L/2$, with $L = 2\pi$—they are oscillations about the potential maxima. Three trajectories are shown (in black lines). One starting from $x = -L$ goes directly to the nearest attractor solution $x_0(t)$. The other two start very near the time-reversed solution $\widetilde{x}(t)$, one within 0.006% and another within $10^{-4}$% from it. After following the time-reversed solution for a few time periods—the closer they initially are to the time-reversed solution, the longer they follow it—both eventually fall into the stable attractors $x_0(t)$.

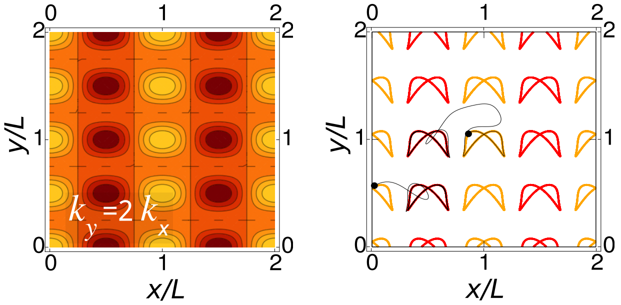


FIG. S2. Instability of the time-reversed solution in a deterministic 2D overdamped system. The potential is $U(x,y) = U_0 \cos(k_x x)[1 + \cos(k_y y)]$, which is shift-symmetric in the $x$-direction, $U(x + L/2, y) = -U(x,y)$, with $L = 2\pi/k_x$. The drive $\mathbf{F}(t) = A[\cos(\omega t)\mathbf{e}_x + \cos(2\omega t + \pi/2)\mathbf{e}_y]$ is anti-symmetric. Reduced units are defined such as $m = k_x = \omega = 1$. Other parameters are $k_y = 2k_x$, $U_0 = \gamma = 50$, $A = 2\gamma$ and $\Gamma = 0$. The left panel depicts a contour plot of the potential landscape. The right panel shows two trajectories (black lines), starting from the filled circles. One goes directly to an attractor solution $\mathbf{r}_0(t) = (x_0(t), y_0(t))$ (the red lines) centered at the potential minima, and the other, starting very near a time-reversed solution $\widetilde{r}(t) = (x_0(-t+\pi) + L/2, y_0(-t+\pi))$ (in yellow)—which are centered about the potential maxima—is able to almost complete a cycle, but before that it falls into an attractor $\mathbf{r}_0(t)$.

## III. The hidden symmetries in a 2D overdamped system

The symmetries (S.2)–(S.3) also hold in higher-dimensions overdamped systems provided the rectification mechanism involves one spatial dimension only. This is illustrated in Figs. S3 and S4 for two-dimensional systems in the overdamped regime.

Figure S3 shows the current in the direction of an applied biharmonic force—the $y$-direction,

$$\mathbf{F}(t) = A[\cos(\omega t) + \cos(2\omega t + \phi)]\mathbf{e}_y, \quad \text{(S.43)}$$

as a function of the driving phase $\phi$. For $\phi = \pi/2$ the driving is anti-symmetric, that is, $\mathbf{F}(-t+\pi/\omega) = -\mathbf{F}(t)$. The system is spatially symmetric in the direction of the applied force. Two specific examples are shown: a system with potential

$$U(x,y) = U_0 \cos(kx)[1 + \cos(3ky)], \quad \text{(S.44)}$$

which is also spatially symmetric in the perpendicular direction—the $x$-direction—and another system with

$$U(x,y) = -U_0 \left[\sin(kx) + \frac{1}{4}\sin(2kx)\right][1 + \cos(2ky)], \quad \text{(S.45)}$$

which is spatially asymmetric in the perpendicular direction. In all cases shown in Fig. S3, the current is suppressed when the driving is anti-symmetric, in agreement

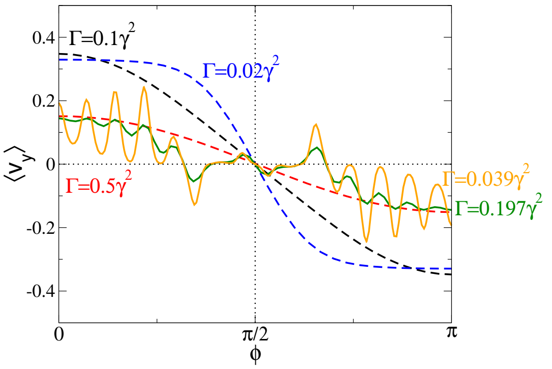


FIG. S3. Current in the direction of an applied biharmonic force (S.43) in a two-dimensional, overdamped system which is spatially symmetric among that direction. The driving (S.43) is anti-symmetric when $\phi = \pi/2$. Reduced units are defined such that $m = k = \omega = 1$. The dashed lines show the current for several values of the noise strength $\Gamma$ for a system with potential (S.44) ($U_0 = \gamma = 50$, $A = 2\gamma$), which is spatially symmetric in the perpendicular direction. The solid lines show the current for the potential (S.45) ($U_0 = \gamma = 50$, $A = 6\pi\gamma$), which is spatially asymmetric in the perpendicular direction.

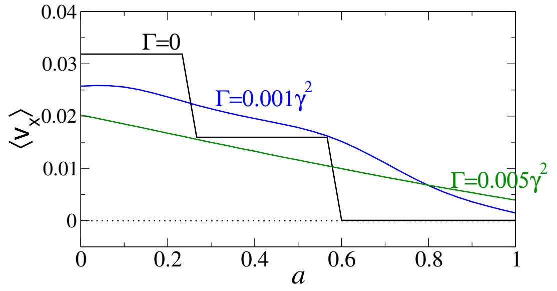


FIG. S4. Current as a function of the symmetry parameter $a$ for several values of the noise strength $\Gamma$ in a two-dimensional, overdamped system. The driving force, given by (S.46), is shift-symmetric by construction, and applied in the $x$-direction only. The potential is (S.47), which is spatially asymmetric for any value of $a$, but shift-symmetric for $a = 1$. Reduced units are defined such that $m = L = 10\omega = 1$. Other parameters are $\gamma = U_0 = 50$ and $A = \gamma$.

with the prediction based on the symmetries (S.2)–(S.3) of one-dimensional systems.

The above scenario is modified whenever more than one degree of freedom takes part to the dynamics, i.e. for higher dimensional systems. In this case, the symmetries (S.2)–(S.3), are not necessarily expected to hold. Such a change in scenario, as determined by a change in the number of degrees of freedom, is illustrated in Fig. S4. In this case a shift-symmetric, periodic drive is applied in the $x$-direction, defined by

$$\mathbf{F}(t) = \begin{cases} \mathbf{F}_d \equiv A[\sin(\omega t) + \sin(2\omega t)]\mathbf{e}_x & \text{first half period} \\ -\mathbf{F}_d(t - \tau/2) & \text{second half period} \end{cases} \tag{S.46}$$

where $\tau = 2\pi/\omega$ is the period. The potential is spatially asymmetric in the $x$-direction,

$$U(x, y) = U_\mathrm{a}(x)\,[1 + \cos(2ky)]\,/(2\pi), \tag{S.47}$$

where $U_\mathrm{a}(x) = U_\mathrm{r}(x)(1 - a) + U_\mathrm{s}(x)a$ is a linear combination of the archetypical ratchet potential

$$U_\mathrm{r}(x) = -\frac{U_0}{2\pi}\left[\sin(kx) + \frac{1}{4}\sin(2kx)\right], \tag{S.48}$$

and $U_\mathrm{s}(x)$ a shift-symmetric potential built from the former,

$$U_\mathrm{s}(x) = \begin{cases} U_\mathrm{r}(x) & \text{first half period} \\ -U_\mathrm{r}(x - L/2) & \text{second half period} \end{cases} \tag{S.49}$$

where $L = 2\pi/k$ is the spatial period in the $x$-direction. Figure S4 depicts the current for several values of the noise strength parameter $\Gamma$. In the deterministic case ($\Gamma = 0$), the current vanishes for a shift-symmetric potential ($a = 1$), as expected in a one-dimensional overdamped system from the symmetries (S.2)–(S.3). However, a finite level of noise makes the system explore the perpendicular direction, inducing a nonzero current for $a = 1$. Despite this fact, the current does not display a component in the perpendicular direction, i.e. $\langle v_y \rangle = 0$ for all values shown in the figure—there is also no current in the perpendicular direction for the examples shown in Fig. S3. Though not strictly satisfied, the effect of the symmetries (S.2)–(S.3) is clearly noticeable in Fig. S4, with a significant suppression of the current at low noise level for a shift-symmetric potential ($a = 1$).

## IV. CONTROL OF TRANSPORT AT THE NANOSCALE AROUND SYMMETRY POINTS

At a symmetry point, the directed current is suppressed. From this point, a small, symmetry-breaking change of the system parameters will induce a non-zero current. By assuming continuity, a similar small change in the opposite direction will also induce a non-zero current, but in the reversed direction, as illustrated in Figs. 1 and 3 with $a$ and $\phi$ as the control parameters, respectively. Therefore, the amplitude and direction of the ratchet current can be precisely controlled around a symmetry point.

The new symmetries thus provide an additional handle of control of transport in periodic potential landscapes. Since they are rigorously satisfied in overdamped systems, typical setups displaying overdamped dynamics, such as colloidal particles [4–12] or driven vortex lattices [13–18] are good candidates for the experimental verification of these symmetries.

The symmetry illustrated in Fig. 3 requires a spatially symmetric system with an anti-symmetric driving force. Since spatial symmetry is not difficult to implement in a large variety of periodic nano-structures, this symmetry can be demonstrated by using, for example,

a bi-harmonic ac-drive, which allows precise control of anti-symmetry—as shown in Fig. 3. Indeed, this procedure was already successfully applied in the experimental control of magnetic flux quanta in nanofabricated devices [19]. In addition, our theoretical explanation guarantees the presence of a current reversal for anti-symmetric driving in other experimental setups.

Note that before the present work, it was believed that anti-symmetric drives yielded current suppression only in shift-symmetric potential landscapes, which are generally more difficult to generate experimentally than spatially symmetric ones. Nevertheless, shift-symmetric potentials for particles at the nanoscale can nowadays be easily generated using lasers. Since the Fourier expansion of shift-symmetric functions contains odd harmonics only, any potential that is a linear combination of odd harmonics is guaranteed to be shift-symmetric. Figure S5 shows an example system. The symmetry is controlled by the mixing parameter $a$ via the potential

$$U(x) = -U_0[\sin(kx) + 0.25\sin(2kx)(1-a) -0.15\cos(3kx)a]. \quad \text{(S.50)}$$

This periodic potential can be easily generated for colloidal particles using optical tweezers [12].

Additionally, the current reversal induced by the hidden symmetry is not restricted to the overdamped regime. A small friction simply shifts the position of the current reversal. As shown in Fig. S5, a current reversal is also expected in weakly damped systems when the mixing parameter $a$ is varied. Therefore, the same procedure could also be applied in cold atoms setups [20–25] to control the amplitude and direction of the atomic current via changes in the optical potential.

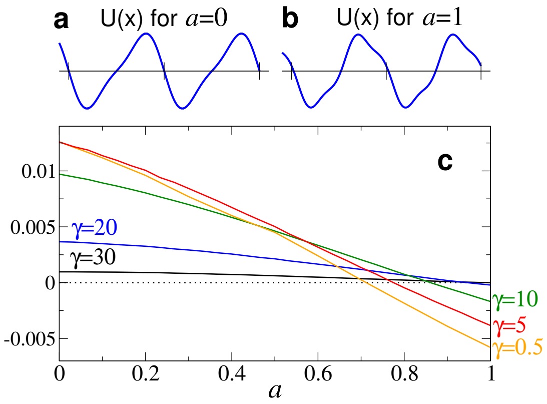


FIG. S5. Same as in Fig. 1 but for a system with a shift-symmetric potential $U_{ss}(x) = -U_0[\sin(kx) - 0.15\cos(3kx)]$ and driving force $F(t) = A[\sin(\omega t) - 0.15\cos(3\omega t)]$ that are easy to generate at the nano or micro-scale using lasers. Rest of the parameters as in Fig. 1.


[1] H. Risken, *The Fokker-Planck Equation* (Springer, Berlin, 1984).
[2] P. Reimann, Phys. Rep. **361**, 57 (2002).
[3] P. Hänggi and F. Marchesoni, Rev. Mod. Phys. **81**, 387 (2009).
[4] J. Rousselet, L. Salome, A. Ajdari, and J. Prost, Nature **370**, 446 (1994).
[5] J. S. Bader, R. W. Hammond, S. A. Henck, M. W. Deem, G. A. McDermott, J. M. Bustillo, J. W. Simpson, G. T. Mulhern, and J. M. Rothberg, Proc. Natl. Acad. Sci. U.S.A. **96**, 13165 (1999).
[6] C. F. Chou, O. Bakajin, S. W. P. Turner, T. A. J. Duke, S. S. Chan, E. C. Cox, H. G. Craighead, and R. Austin, Proc. Natl. Acad. Sci. U.S.A. **96**, 13762 (1999).
[7] A. van Oudenaarden and S. G. Boxer, Science **285**, 1046 (1999).
[8] S. Matthias and F. Müller, Nature **424**, 53 (2003).
[9] L. Faucheux, L. Bourdieu, P. Kaplan, and A. Libchaber, Phys. Rev. Lett. **74**, 1504 (1995).
[10] S.-H. Lee, K. Ladavac, M. Polin, and D. G. Grier, Phys. Rev. Lett. **94**, 110601 (2005).
[11] A. V. Arzola, K. Volke-Sepulveda, and J. L. Mateos, Phys. Rev. Lett. **106**, 168104 (2011).
[12] O. Marago, P. Jones, P. Gucciardi, G. Volpe, and A. Ferrari, Nat. Nano. **8**, 807 (2013).
[13] C.-S. Lee, B. Jankó, I. Derényi, and A.-L. Barabási, Nature **400**, 337 (1999).
[14] D. Shalóm and H. Pastoriza, Phys. Rev. Lett. **94**, 177001 (2005).
[15] J. Wambaugh, C. Reichhardt, C. Olson, F. Marchesoni, and F. Nori, Phys. Rev. Lett. **83**, 5106 (1999).
[16] J. Villegas, S. Savel'ev, F. Nori, E. Gonzalez, J. Anguita, R. Garca, and J. Vicent, Science **302**, 1188 (2003).
[17] D. Cole, S. Bending, S. Savel'ev, A. Grigorenko, T. Tamegai, and F. Nori, Nature mat. **5**, 305 (2006).
[18] C. de Souza Silva, J. V. de Vondel, M. Morelle, and V. Moshchalkov, Nature **440**, 651 (2006).
[19] S. Ooi, S. Savel'ev, M. B. Gaifullin, T. Mochiku, K. Hirata, and F. Nori, Phys. Rev. Lett. **99**, 207003 (2007).
[20] C. Mennerat-Robilliard, D. Lucas, S. Guibal, J. Tabosa, C. Jurczak, J.-Y. Courtois, and G. Grynberg, Phys. Rev. Lett. **82**, 851 (1999).
[21] M. Schiavoni, L. Sanchez-Palencia, F. Renzoni, and G. Grynberg, Phys. Rev. Lett. **90**, 094101 (2003).
[22] R. Gommers, S. Bergamini, and F. Renzoni, Phys. Rev. Lett. **95**, 073003 (2005).
[23] R. Gommers, S. Denisov, and F. Renzoni, Phys. Rev. Lett. **96**, 240604 (2006).
[24] D. Cubero, V. Lebedev, and F. Renzoni, Phys. Rev. E **82**, 041116 (2010).
[25] A. Wickenbrock, P. C. Holz, N. A. A. Wahab, P. Phoonthong, D. Cubero, and F. Renzoni, Phys. Rev. Lett. **108**, 020603 (2012).
